# Supplementary material for: FVH-Bench: Evaluating Image Generator Safety Beyond Overtly Harmful Imagery
Source: arXiv:2610.37722 source file (2026-12-03)
Supplement: Supplementary file 1 [file benign_controls_table.tex]

\begin{tabular*}{\linewidth}{@{\extracolsep{\fill}}lrr@{}}
\toprule
\textbf{Visual form} & \textbf{Count} & \textbf{Share (\%)} \\
\midrule
Guides, diagrams and maps & 46 & 23.0 \\
Educational infographics & 16 & 8.0 \\
Comics & 10 & 5.0 \\
Interfaces and dashboards & 28 & 14.0 \\
Documents, records and schedules & 30 & 15.0 \\
Notices, newsletters and event posters & 40 & 20.0 \\
Menus and product catalogs & 20 & 10.0 \\
Everyday scenes & 10 & 5.0 \\
\midrule
Total & 200 & 100.0 \\
\bottomrule
\end{tabular*}
